# Supplementary material for: Robust Human Registration with Body Part Segmentation on Noisy Point Clouds
Source: arXiv:2504.03602 source file (2025-04-04)
Supplement: Supplementary file 1 [file 06_supplementary.tex]

\begin{table}[H]
\centering
\scriptsize
\caption{Video Fitting}
\begin{tabular} {l@{\hskip 8pt}ccccc@{\hskip 8pt}}
\toprule
\textbf{Metric} & \textbf{Dance} & \textbf{Fight} & \textbf{Pose} & \textbf{Sidehug} & \textbf{Weighted Average} \\
\midrule
\textbf{Sequential} \\
\text{Time [s]} & 1.482 & 1.965 & 1.286 & 1.730 & 1.622 \\
\text{V2V [mm]} & 20.3 & 25.8 & 21.7 & 27.1 & 23.8 \\
\text{J2J [mm]} & 19.5 & 21.2 & 18.1 & 22.0 & 20.3 \\
\midrule
\textbf{Individual} \\
\text{Time [s]} & 1.852 & 1.989 & 1.768 & 1.723 & 1.827 \\
\text{V2V [mm]} & 21.1 & 24.1 & 22.6 & 29.9 & 24.7 \\
\text{J2J [mm]} & 19.7 & 19.8 & 19.5 & 23.4 & 20.8 \\
\midrule
\textbf{Number of Humans} & 56 & 42 & 38 & 58 & - \\
\bottomrule
\end{tabular}
\label{tab:video_fitting}
\end{table}

\begin{figure}[h]
    \centering
    \includegraphics[width=0.8\textwidth]{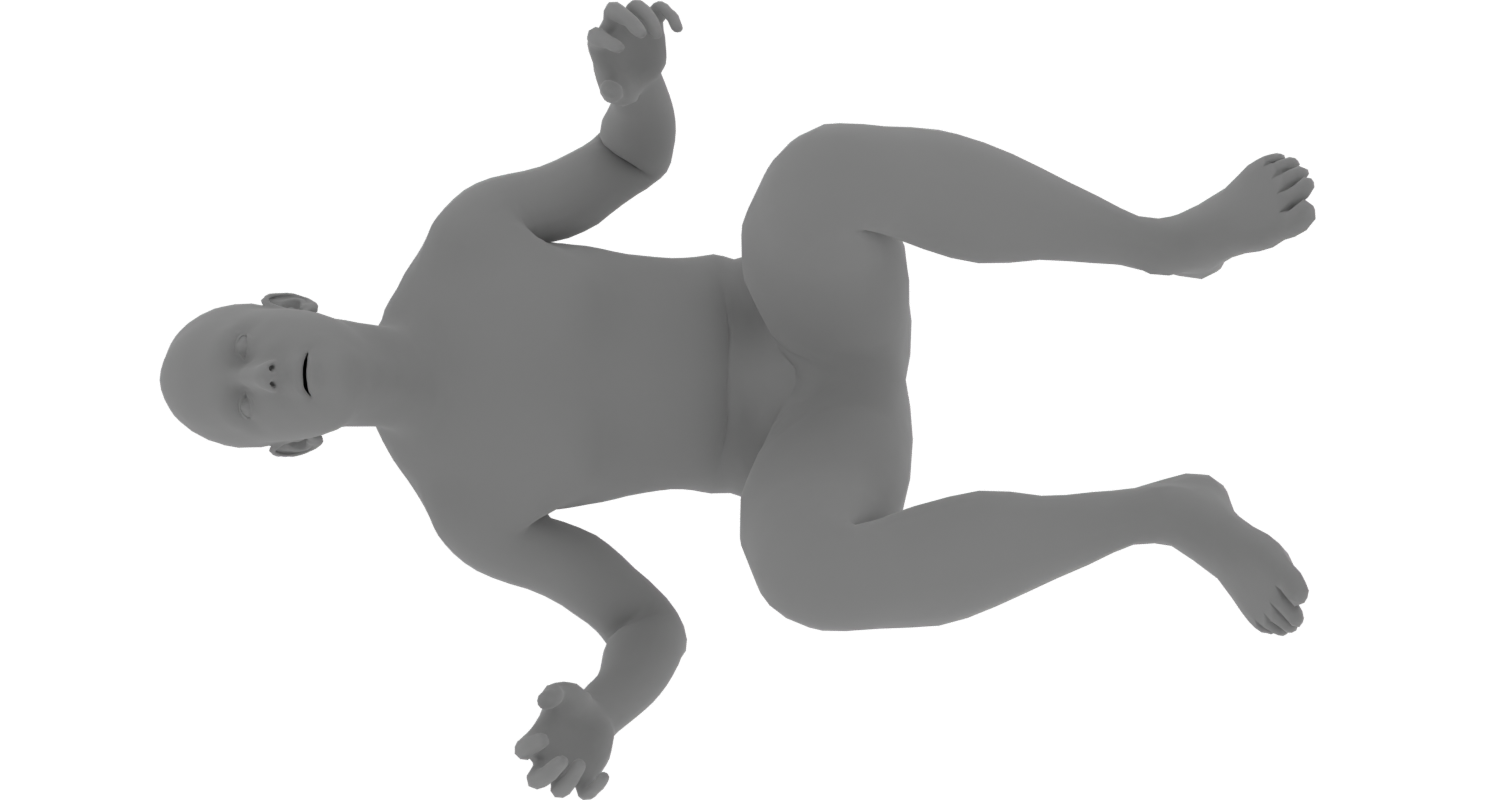}
\end{figure}

\section{Training Details}
on which dataset are they trained?
